# Supplementary material for: PERFOGRAPH: A Numerical Aware Program Graph Representation for Performance Optimization and Program Analysis
Source: arXiv:2306.00210 source file (2023-11-30)
Supplement: Supplementary file 1 [file supplementary.tex]

% Hyperparamter tuning
% Datasets
% Ablation
% Kernel-wise stats 
% IR2vec transfer here from device mapping
